# Supplementary material for: Reorientation of the stripe Phase of 2D Electrons by a Minute Density Modulation
Source: arXiv:1607.05744 source file (2016-07-21)
Supplement: Supplementary file 1 [file Supplementary.pdf]

# Supplemental Material to "Reorientation of the stripe Phase of 2D Electrons by a Minute Density Modulation"

M. A. Mueed, Md. Shafayat Hossain, L. N. Pfeiffer, K. W. West, K. W. Baldwin, and M. Shayegan
*Department of Electrical Engineering, Princeton University, Princeton, New Jersey 08544, USA*
(Dated: June 8, 2016)

This Supplemental Material describes two different methods to quantify the amplitude of the external modulation imposed on the two-dimensional electron system (2DES) confined to a 30-nm-wide GaAs quantum well. The analysis presented here demonstrates that the amplitude of such modulation is minute.

The external modulation stems from a strain-inducing superlattice patterned on the surface of our samples. The superlattice, made of negative electron-beam resist, imparts a density modulation of the same period to the 2DES through the piezoelectric effect in GaAs [1–6]. In Fig. S1, we show magnetoresistance data, taken at *zero* parallel field ($B_{||}$) and small perpendicular field ($B_\perp$), that allow us to estimate the strength of the external periodic modulation at $B_{||} = 0$. Three such traces for different modulation periods are included in the figure. In a density-modulated 2DES, a resistivity minimum occurs whenever the electron's cyclotron diameter ($2R_c$) becomes commensurate with the modulation period $a$. This leads to magnetoresistivity oscillations, known as commensurability oscillations (COs), at low $B_\perp$ [1–11]. We observe such oscillations in Fig. S1 for $a = 200$ and 150 nm. The amplitude of COs ($\rho_{co}^{osc}$) depends on $\eta$, defined as the ratio of the external modulation amplitude to the Fermi energy $E_F$.

Using a perturbative model we can express $\rho_{co}^{osc}$, normalized to the *zero* field resistivity $\rho^o$, as a function of $\eta$ [1–6]:

$$\frac{\rho_{co}^{osc}}{\rho^0} = A(\frac{\pi}{\omega_c \tau_{co}})\frac{\eta^2}{2}\frac{L}{a}\mu B \sin(2\pi\frac{2R_c}{a}) \qquad (1)$$

$\rho_{co}^{osc}$ also depends on the mean-free-path $L = \hbar k_F \mu/e$, where $\mu$ is the mobility and $k_F$ is the Fermi wavevector, and a damping factor $A(\pi/\omega_c\tau_{co})$ [4, 6] where $\omega_c$ is the cyclotron frequency and $\tau_{co}$ is the CO lifetime. This damping factor, defined as $A(x) = x/\sinh(x)$, takes into account scattering events that occur as the electron is completing a cyclotron orbit. One method of estimating $\eta$ is to fit the observed COs using equation 1.; the dotted red curve in Fig. S1 shows such a fit for the $a = 200$ nm data, yielding $\eta \simeq 1\%$. $\eta$ can also be extracted from the extinction field $B_E$ according to the expression: $B_E = \eta(\pi\hbar\sqrt{2\pi n}/ae)$ [4–6, 11]. When $B_\perp > B_E$, the Lorentz force on the electrons becomes sufficiently large to overcome the potential barrier created by the external modulation, thus decreasing the resistivity and resulting in a positive magnetoresistivity peak at $B_E$ (marked by vertical arrows in Fig. S1).

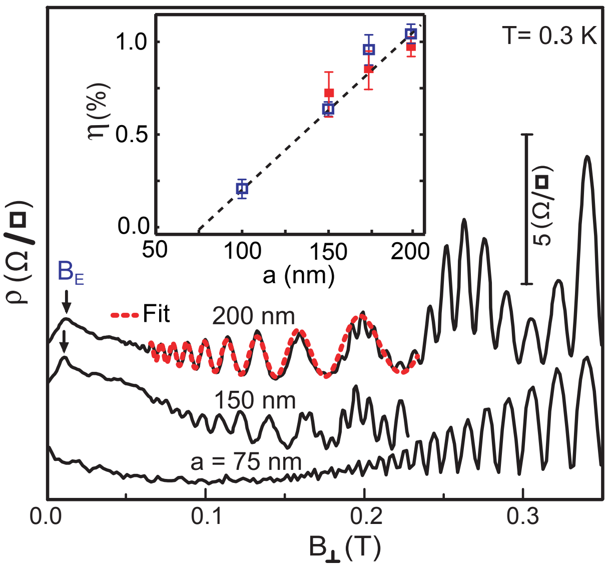


FIG. S1. Magnetoresistivity traces of the patterned regions for $a = 200$, 150, 75 nm. While both $a = 200$ and 150 nm traces show pronounced COs (highlighted by the red curve in the $a = 200$ nm trace) at small $B_\perp$, the $a = 75$ nm trace shows none. We also observe Shubnikov de Hass oscillations at $B_\perp \gtrsim 0.2$ T in all three traces. The fit of the COs (red dotted curve) provides a measure of the external density modulation strength, $\eta$ (see text). The extinction field $B_E$ (marked by the vertical arrow) also gives an estimate of $\eta$ (see text). Inset: $\eta$ as a function of the modulation period $a$. The red and blue squares correspond to values of $\eta$ estimated from the fit and positions of $B_E$, respectively. Note that the dashed line, which is a guide to the eye, extrapolates to $\eta \simeq 0$ for $a = 75$ nm, consistent with the absence of COs or an extinction field in the experimental data (lowest trace).

We plot $\eta$ as a function of $a$ in Fig. S1 inset. It is clear that $\eta$ decreases with decreasing $a$. For shorter periods, as their ratio to the 2DES depth from the surface becomes smaller, the higher harmonics of the potential modulation are attenuated, resulting in a weaker amplitude [3, 6, 12, 13]. For the $a = 75$ nm trace, we cannot estimate $\eta$ using the above methods since no COs or $B_E$-feature are observed. However, from its dependence on $a$, we conclude that $\eta < 0.25\%$. Such a weak modulation is consistent with the fact that $a = 75$ nm is significantly smaller than our sample's 2DES depth (135 nm).

[1] R. Cusco, M. C. Holland, J. H. Davies, I. A. Larkin, E. Skuras, A. R. Long, and S. P. Beaumont, Surf. Sci. **305**, 643 (1994).

[2] E. Skuras, A. R. Long, I. A. Larkin, J. H. Davies, and M. C. Holland, Appl. Phys. Lett. **70**, 871 (1997).

[3] A. R. Long, E. Skuras, S. Vallis, Ramon Cusco, Ivan A. Larkin, John H. Davies, and M. C. Holland, Phys. Rev. B **60**, 1964 (1999).

[4] A. Endo, S. Katsumoto, and Y. Iye, Phys. Rev. B **62**, 16761 (2000).

[5] A. Endo and Y. Iye, Phys. Rev. B **72**, 235303 (2005).

[6] D. Kamburov, H. Shapourian, M. Shayegan, L. N. Pfeiffer, K. W. West, K. W. Baldwin and R. Winkler, Phys. Rev. B **85**, 121305(R) (2012).

[7] D. Weiss, K. von Klitzing, K. Ploog, and G. Weimann, Europhys. Lett. **8**, 179 (1989).

[8] R. R. Gerhardts, D. Weiss, and K. von Klitzing, Phys. Rev. Lett. **62**, 1173 (1989).

[9] R. W. Winkler, J. P Kotthaus, and K. Ploog, Phys. Rev. Lett. **62**, 1177 (1989).

[10] C. W. J. Beenakker, Phys. Rev. Lett. **62**, 2020 (1989).

[11] P. H. Beton, E. S. Alves, P. C. Main, L. Eaves, M. W. Dellow, M. Henini, O. H. Hughes, S. P. Beaumont, and C. D. W. Wilkinson, Phys. Rev. B **42**, 9229 (1990).

[12] John H. Davies and Ivan A. Larkin, Phys. Rev. B **49**, 4800 (1994).

[13] J. P. Lu, X. Ying and M. Shayegan, Appl. Phys. Lett. **65**, 2320 (1994).
